# Supplementary material for: Autonomous Catheterization with Open-source Simulator and Expert Trajectory
Source: arXiv:2401.09059 source file (2024-01-20)
Supplement: Supplementary file 1 [file 7_appendix.tex]

% \section{CathSim Design Details}
% \label{app_cathsim_design}

% \begin{figure}[h]
% 	\centering
  
%     \subfigure[The design of the Robotic Follower (Slave Robot)\label{subfig:cathbot}]{\includegraphics{assets/cathbot-follower.drawio.pdf}} \hfill
%     \subfigure[Our simulated version of the Robotic Follower]{\includegraphics[width=0.45\textwidth]{assets/cathbot_sim.png}} 
%     \vspace{-1ex}
% 	\caption{Schematic representation of the CathBot's follower mechanism~\citep{kundrat2021mr} (a) alongside a visualization of our simulated model (b).}
% 	\label{fig:follower}
% \end{figure}

% \textbf{Robotic Follower.} In our study, we focus on simulating the robotic follower, predicated on the linear relationship between the leader and follower, as outlined in the CathBot design \citep{kundrat2021mr}. For the sake of simplicity, our simulation comprises four modular platforms attached to the main rail; two of these platforms hold the guidewire during translational movements with clamps, while the other two facilitate angular movements via rotary catheter and guidewire platforms. Prismatic joints connect the main rail components and the clamps, enabling translational movements, while revolute joints link the wheels, allowing the catheter and guidewire to rotate~(refer to Fig.~\ref{fig:follower} for the design).

% \textbf{Actuation.} CathBot's actuation entirely depends on the frictional forces $f_f$ between the guidewire and the clamp. In our simplified model, we assert that the frictional force $f_f$ is sufficient to entirely prevent slippage ($f_f \geq f_s$), hence eliminating the need to account for the effects of sliding friction $f_s$. This approach gives us direct control over the joints without having to simulate frictional effects, leading to faster simulation times due to fewer contact points. Furthermore, a friction-based actuation mechanism could potentially slow down execution times and increase error probability due to simulation noise. Thus, we argue that our choice to assume perfect motion results in enhanced computational efficiency, particularly within the context of our defined problem domain.

% \textbf{Aortic Models.} In addition to Type-I Aortic Arch model which is mainly used in our experiments, we incorporate three distinct aortic models to enrich our anatomical dataset. These models include a high-fidelity Type-II aortic arch and a Type-I aortic arch with an aneurysm, both sourced from Elastrat, Switzerland. Furthermore, a low tortuosity aorta model, based on a patient-specific CT scan, is included. With these three additional representations, our simulator contains four distinct aorta models. These models aim to enhance the diversity and accuracy of aortic structures available for research and educational endeavors. These aortas are visualized in Fig.~\ref{fig:three aorta}.

% \begin{figure}[ht]
%     \centering
%     \subfigure[Type-I (Aneurysm)]{%
%         \includegraphics[width=0.3\textwidth]{assets/rebuttal/aneurysm.png}
%         \label{fig:five over x}
%     }\hfill
%     \subfigure[Type-II]{%
%         \includegraphics[width=0.3\textwidth]{assets/rebuttal/type2.png}
%         \label{fig:type2}
%     }
%     \hfill
%     \subfigure[Low Tortuosity]{%
%         \includegraphics[width=0.3\textwidth]{assets/rebuttal/low_tort.png}
%         \label{fig:three sin x}
%     }
%     \caption{Aortic Models.}
%     \label{fig:three aorta}
% \end{figure}


% \section{CathSim Speed Evaluation}
% \label{app_speed_evaluation}

% \begin{minipage}[t]{\textwidth}
%     \begin{minipage}[t][][b]{0.5\textwidth}
%         \adjustimage{left}{assets/episode_time.png}
%         \captionof{figure}{CathSim training speed.}
%         \label{fig:fps}
%     \end{minipage}
%     \hfill
%     \begin{minipage}[t][][b]{0.47\textwidth}
%         \begin{minipage}[t]{\textwidth}
%             \vspace{0.35cm}
%             \scriptsize
%             \centering
%             \input{tables/training_times_coparison}
%         \end{minipage}
%     \end{minipage}
% \end{minipage}

% \textbf{Training Speed.} As illustrated in Fig.~\ref{fig:fps}, we provide a comparison of frames per second (FPS) for the various algorithms we employed during model training. It is evident that utilizing solely the internal state space, comprised of joint positions and velocities, facilitates expedited training processes. In contrast, integrating all modalities into the training process results in its deceleration. The most significant computational demand arises from the dual convolutional neural networks utilized in both the image and mask representations. However, despite this load, the algorithms exhibit respectable computational speed, even during the training phase. Our simulator supports approximately $40$ to $80$ frames per second performance for all implemented algorithms, underscoring the computational speed of our simulation environment. Moreover, we provide the training times in terms of hours for the different modalities in Table~\ref{tab:training-time}.

% \section{Evaluation Metrics}
% \label{app_evaluation_metric}

% \textbf{Force.} In our study, the force applied by surgical instruments during the simulation is critical for evaluating their performance and interaction with the aorta. To accurately record this force, we used a manual cannulation method through our simulator. At each time step of the simulation, we collected the collision points between the guidewire and the aorta. These collision points give us crucial insights into the tridimensional force acting on the system, which consists of the normal force (\(f_z\)) and the frictional forces (\(f_x\) and \(f_y\)). To compute the total magnitude of the force, we calculated the Euclidean norm of the force vector at a given time step (\(t\)), denoted as \(f_t\). This magnitude is obtained from the square root of the sum of the squares of the force vector components 

% \begin{equation}
%     f_t = \sqrt{ f_{x,t}^2 + f_{y,t}^2 + f_{z,t}^2}\label{eq:force}
% \end{equation}


% This allows us to holistically assess the collective impact of the force components, providing a more comprehensive understanding of the guidewire's behavior and its interaction forces with the aorta throughout the simulation. Furthermore, it facilitates a comparison between our experiments and those conducted by~\citet{kundrat2021mr}.

% \textbf{Path Length.} The path length was derived by summing the Euclidean distances between sequential positions of the guidewire head. For each time step, the position of the guidewire head, denoted as \(h_{t}\), was extracted. The Euclidean distance between the guidewire head position at time \(t\) and the position at time \(t+1\), denoted as \(h_t\) and \(h_{t+1}\) respectively, was then calculated \(d(h_{t}, h_{t+1}) = \sqrt{(h_{t+1} - h_{t})^2}\). This process resulted in a path length represented by:
% \begin{equation}
%     \operatorname{Path Length} = \sum\limits_{i=1}^n||h_{t+1} - h_{t}||
% \end{equation}
% where \(n\) is the episode length.

% \textbf{SPL.} The navigation performance of the expert was evaluated in relation to human performance. This involved utilizing the path length, as calculated in the previous paragraph, to assess the optimality of the navigation. An optimal policy results in the shortest path. The Success Weighted by Normalized Inverse Path Length (SPL) metric, as suggested by~\citet{anderson2018evaluation} was then computed using 
% \begin{equation}
%     \operatorname{SPL}=\frac{1}{N} \sum\limits_{i=1}^N S_i\frac{l_i}{\max(p_i,l_i)}
% \end{equation}
% where the path length \(p_i\) is normalized by the optimal path \(l_i\). In this context, the shortest path observed was used as the optimal path, considering that human performance is consistently outperformed by the RL policies. 

% \textbf{Safety.} We compute the safety based on the number of times an algorithm inflicts a force greater than \(2\unit{\newton}\). This constant is derived from the study in real-world setup~\citep{kundrat2021mr}. As such, we create a binary variable \(a\in\{0,1\}\) where \(a=1\) if \(f_t \geq 2\unit{\newton}\). As such, the safety metric is defined as:

% \begin{equation}
%     \operatorname{Safety} = 1 - \frac{1}{N} \sum_{i=1}^N a_i
% \end{equation}
% where \(N\) represents the number of steps within an episode. We further subtract the result from \(1\). Intuitively, an algorithm that inflicts a great force at each step during the episode will have a safety of \(0\%\), whereas an algorithm that inflicts a damage of \(f \leq 2\unit{\newton}\) at all time steps, will result in a safety of \(100\%\). 

% \textbf{Episode Length.} The length of an episode is determined by the number of steps an algorithm takes to complete a task. This metric is significant as it provides insight into the efficiency of an algorithm; fewer steps generally indicate more efficient performance, assuming that the quality of task completion is preserved.

% \textbf{Success.} The success of an episode is defined by whether the agent is able to achieve the goal within a pre-specified time limit of \(300\) time steps. This metric is binary; it records a success if the goal is reached within the time limit, and a failure otherwise. This serves to measure the effectiveness of the agent in task completion under time constraints, mirroring real-world scenarios where timeliness is often crucial.

% \section{CathSim Validation Against Real-Robot}
% \label{app_cathsim_real_robot}

% \textbf{Force Extraction.} The real robot experiments conducted by~\citet{kundrat2021mr} employed a 6 DoF force sensor (Mini40, ATI Industrial Automation, Apex, USA) to measure the force produced by the interaction between the instruments and the silicone phantom~(see Fig.~\ref{fig:cathbot-experiment_setup}). The force sensor was placed directly underneath the phantom, where the magnitude of the force was extracted. Similarly, in order to extract the force within our simulator, we manually carry out the cannulation using an input device and extract the forces at each time step. For each simulation time step, we extract the collision points between the guidewire and the aorta, along with the tridimensional force expressed as the normal force $f_z$ and frictional forces $f_x$ and $f_y$. We then compute the force magnitude using Equation~\ref{eq:force}.


% \begin{figure}[h]
%     \centering
%     \includegraphics{assets/cathbot-experiment_setup.pdf}
%     \caption{Experimental setup of CathBot: (1) Pulsatile and continuous flow pumps, (2) Force Sensor, (3) Vascular phantom, (4) Webcam, (5) NDI Aurora field generator, (6) Catheter manipulator (i.e., robotic follower), (7) Simulated X-ray Screening, and (8) Master device. Adapted from~\citet{chi2020collaborative,kundrat2021mr}.}
%     \label{fig:cathbot-experiment_setup}
% \end{figure}

% \textbf{Distribution Comparison.} We begin our comparison with the Shapiro-Wilk test of normality on the data extracted from the simulator and, given a p-value of $p \approx 7.195\times 10^{-17}$ and a statistic of $0.878$, we conclude that the sampled data does not represent a normal distribution ${\mathcal{N}}(\mu, \sigma)$. Furthermore, we assess the homoscedasticity of the sample distribution and normal distribution by using Levene's tests, which results in a statistic of $40.818$ and a p-value of $p\approx 2.898\times 10^{-10}$, therefore, concluding that $\sigma_1^2 \neq \sigma_2^2$. Given the previous statistics (i.e., non-normal distribution and unequal variances), we select the non-parametric Mann-Whitney test to compare the given distributions. The statistical tests show that our CathSim can mimic the real-robot behavior, as indicated in the main paper.

% The resulting statistic given the test is $76076$, with a p-value of $p\approx0.445$. Given that the p-value is higher than the threshold of $p=0.05$, we can conclude that the differences in the distributions are merely given to chance and therefore the distributions can be considered as being part of the same population and thus convene that the force distribution of our simulator closely represents the distribution of forces encountered in the real-life system. Therefore, we can see that our CathSim successfully mimics the behavior of the real-world system.


% \section{Experimental setup}
% \label{app_exp_setup}

%Our simulation framework positions a guidewire as an agent within an episodic, Partially Observable Markov Decision Process (POMDP) environment that is depicted by a Type-I Aortic Arch. The state representation $s_t$ includes a normalized grayscale image \(I\), a segmentation map of the guidewire \(S\), and joint positions \(Q\) and velocities \(V\). The actions reflect real robot movements (\textit{i.e.}, translation and rotation) represented by \(a\). 


% \section{Expert Navigation Network Implementation}
% \label{app_expert_nav}

% \textbf{Observation Space.} We incorporated a range of observations to provide the agent with an extensive understanding of the environment. A grayscale image of dimensions $80 \times 80$ (denoted by \(I \in [0, 1]^{80 \times 80}\)) is generated as a visual clue, which is accompanied by the ground truth binary segmentation mask \(S \in \{0,1\}^{80 \times 80}\). The mask \(S[i,j] = 1\) is validated only when the pixel coordinates \((i,j)\) are part of set \(A\), the pixels that constitute the guidewire. Furthermore, to enhance the reinforcement learning problem's optimization, we also included the ground truth joint positions \(Q \in \mathbb{R}^{168}\) and joint velocities \(V \in \mathbb{R}^{168}\). These joint values provide detailed mechanical insight into the guidewire's state, enriching the agent's knowledge base and facilitating informed decision-making.

% \textbf{Action Representation.} In CathSim, the essential actions are denoted by translation \(a_t \in [-1,1]\) and rotation $a_r \in [-1,1]$. At each time step, the agent generates these actions, which are collectively represented by the vector $a \in [-1,1]^2$. Here, a positive $a_t$ denotes forward movement, while a negative $a_t$ signifies a backward movement. Similarly, a positive $a_r$ corresponds to a clockwise guidewire rotation, while a negative $a_r$ indicates an anticlockwise rotation. The selection of translation and rotation actions in CathSim closely mirrors the actions in real-world endovascular procedures, as described by~\citet{kundrat2021mr}. By faithfully reproducing the motions of an actual robot, the simulation environment better replicates real-world situations. This enables the reinforcement learning agent to acquire policies that can be feasibly implemented in a physical robot, thereby augmenting the practical value and applicability of the behaviors learned.

% \textbf{Reward Function.} Our employed reward system is dense, and it hinges on the spatial position of the guidewire tip in relation to the goal. Formally, the reward $r$ is determined by the function $r(p_t, g)=-d(p_t,g)$, where $d(p_t,g)=||p_t-g||$ characterizes the distance between the position $p$ of the guidewire tip at time $t$ and the target $g$. If the guidewire tip lies within a distance threshold $\delta$ of the target $g$, the agent is conferred a positive reward $r$. For our research, we adopted a $\delta$ of $4\unit{\milli\metre}$ and assigned a task completion reward of $r=10$. Consequently, we end up with the following reward function:

% \begin{equation}
% r(h_t, g) = 
%     \begin{cases}
%     10 & \text{if} \quad d(h,g) \leq \delta \\
%     -d(h,g) & \text{otherwise} 
%     \end{cases}
% \end{equation}

% \textbf{Training Details.} The experiments were conducted on an  NVIDIA RTX 2060 GPU (\(33\unit{\mega\hertz}\)) system on an Ubuntu 22.04 LTS based operating system. Furthermore, the system contained an AMD Ryzen 7 5800X 8-Core Processor with a total of 16 threads with \(64\unit{\giga\byte}\) of RAM. All experiments used PyTorch, whilst for the Soft Actor Critic implementation we used stable baselines~\citep{stable-baselines3}. The training was carried out for a total of $600,000$ time steps using a total of $5$ different random seeds, resulting in a training time bounded between $2$ and $5$~hours. Each episode has two terminal states, one which is time-bound (i.e., termination of an episode upon reaching a number of steps) and one which is goal bound (i.e., the agent achieves the goal $g$).



% \begin{minipage}[t]{\textwidth}
%     % \vspace{-1cm}
%     \begin{minipage}[t][][b]{0.6\textwidth}
%         \centering
%         \scriptsize
%         \input{tables/ENN_architecture}
%     \end{minipage}
%     \hfill
%     \begin{minipage}[t][][b]{0.35\textwidth}
%         \begin{minipage}[t]{\textwidth}
%             \scriptsize
%             \centering
%             \input{tables/ENN_hyperparams}

%         \end{minipage}
%     \end{minipage}
% \end{minipage}

% \textbf{Networks.} We employ multiple feature extractors to dissociate the dominant features within our Expert Navigation Network~(ENN). Specifically, we use a convolutional neural network (CNN~\citep{mnih2015human}) to extract the image-based features, resulting in two latent features $J_I$ and $J_S$ that represent the top camera view and guidewire segmentation map. The CNN is composed of $3$ convolutional layers with a $\operatorname{ReLU}$~\citep{agarap2018deep} activation function, followed by a flattening operation. We also concatenate joint positions~$Q$ and joint velocities~$V$ to generate a joint feature vector $J_J=Q \parallel P$ of dimensionality $336$ which is then passed through the MLP. These features are concatenated to form a single feature vector $J=J_I \parallel J_S \parallel J_J$, which is fed into a policy network $\pi (a_t,\theta)$. Both network architectures are presented in Table~\ref{tab:network-architectures-cnn-mlp}.

% \textbf{SAC.} Our primary reinforcement learning method is the soft actor-critic~(SAC)~\citep{haarnoja2018soft}. Soft actor-critic (SAC) is a model-free reinforcement learning algorithm that learns a stochastic policy and a value function simultaneously. The objective function of SAC combines the expected return of the policy and the entropy of the policy, which encourages exploration and prevents premature convergence to suboptimal policies. The algorithm consists of three networks, namely a state-value function $V$ parameterized by $\psi$, a soft $Q$-function $Q$ parameterized by $\theta$, and a policy $\pi$ parameterized by $\phi$. The parameters we employ are present in Table~\ref{tab:sac}. For the policy network, we use a composition of linear layers to handle and transform the input data.



% \section{Downstream Tasks}
% \label{app_downstream_task}

% \subsection{Imitation Learning}


% \textbf{Network.} The architecture of our network for the Behavioral Cloning (BC) algorithm consists of a sequence of specialized layers that gradually transform the input data. The process initiates with the input, formatted as a tensor of dimensions (1, 80, 80), which is passed through three Conv2D layers. All of these layers employ the Rectified Linear Unit (ReLU) as their activation function. Upon passing through the Conv2D layers, the output tensor is reshaped into a single dimension by a flattening layer, facilitating the shift from convolutional to linear layers. The flattened output is then processed by a Linear layer utilizing the ReLU activation function. Finally, an additional Linear layer, without an activation function, delivers the final output of the network. This last layer provides raw scores, which are interpreted directly as the network's output, mirroring the decisions made by the BC algorithm. The network architecture is illustrated in Table~\ref{tab:bc-network}.


% \begin{minipage}[t]{\textwidth}
%     \begin{minipage}[t][][b]{0.6\textwidth}
%         \centering
%         \scriptsize
%         \centering
%         \scriptsize
%         \input{tables/BC_architecture}
%     \end{minipage}
%     \hfill
%     \begin{minipage}[t][][b]{0.35\textwidth}
%         \begin{minipage}[t]{\textwidth}
%             \scriptsize
%             \centering
%             \input{tables/BC_hyperparams}
%         \end{minipage}
%     \end{minipage}
% \end{minipage}

% \begin{table}[h]

% \end{table}

% \textbf{Training.} To train the BC algorithm, we employ a set of hyperparameters, as listed in Table~\ref{tab:bc-hyperparameters}. The training procedure makes use of a batch size of \(32\). The Adam~\citep{kingma2014adam} optimizer is utilized to minimize the loss function. We set the learning rate and entropy coefficient to \(1 \times 10^{-3}\), controlling the step size at each iteration of the optimization and regularizing the policy towards a more exploratory behavior, respectively. The training process spans over \(800\) epochs, each epoch consisting of a complete pass through the entire dataset, providing the model ample opportunity to converge to an optimal solution.




% \subsection{Force Prediction}

% \input{tables/force_prediction_network}

% \textbf{Network.} We utilize a hybrid architecture comprising a CNN followed by an MLP, with a grayscale image as the input. The network architecture includes three Conv2D layers that apply convolution operations to the input tensor. Each of these convolutional layers employs the Scaled Exponential Linear Unit (SELU~\citep{klambauer2017selfnormalizing}) as the activation function, encouraging self-normalization and improving the network's capability to propagate gradients deeply into the architecture. Subsequent to the Conv2D layers, a flattening layer reshapes the output into a one-dimensional tensor. Thereafter, the architecture implements three Linear layers. The initial two layers use the SELU activation function, while the final one adopts the Rectified Linear Unit (ReLU~\citep{agarap2018deep}) activation function. This amalgamation of multiple linear layers, each paired with a distinct non-linear activation function, enables the network to learn complex patterns in the input data, leading to the network's final output. Table~\ref{tab:force-network} shows the force prediction network architecture.

% \textbf{Training.} We employed the NAdam optimizer~\citep{dozat2016incorporating} to train our model, setting the initial learning rate at \(4\times10^{-4}\). This was coupled with a SELU activation function to enhance self-normalization and facilitate gradient propagation. To dynamically adjust the learning rate during the training process, we used a OneCycle learning rate scheduler~\citep{smith2018superconvergence}, and the training was conducted for a total of \(30\) epochs.

% \textbf{Data Management.} In terms of data management, we divided the original dataset into training, testing, and validation subsets according to the total time steps. Initially, we allocated \(20\%\) of the total time steps to the test set. Subsequently, the remaining data was partitioned into a validation set and training set, with the validation set representing \(20\%\) of the leftover steps. This procedure was followed for each experimental run of our force prediction model, generating corresponding sets of transitions. Of particular note, the test set consistently stemmed from our largest trajectory dataset—the \(100K\) dataset. For each training run, we designated \(20\%\) of this dataset for validation, utilizing the remaining portion for training. The model's performance was assessed using the originally separated test set. By adhering to this structured and consistent methodology, we ensured a rigorous and equitable evaluation of our model's performance across multiple runs.


% \section{Questionnaire}\label{app_questionaire}

% The study was conducted with ten volunteer participants to evaluate the effectiveness and authenticity of our endovascular simulator. These participants, who had no prior experience in endovascular navigation, provided feedback using a 5-point Likert scale~\citep{likert1932technique}. Initially, participants were shown an actual endovascular navigation fluoroscopic video. Following this, they directly interacted with the simulator, tasked with cannulating two targets: the brachiocephalic artery and the left common carotid artery. Upon task completion, participants filled out a questionnaire featuring the following prompts:

% \begin{enumerate}
% \item How well did the simulator simulate the anatomy and structure of blood vessels?
% \item How closely did the simulator replicate the visual experience of navigating a real endovascular procedure?
% \item How satisfied were you with the overall performance and functionality of the simulator?
% \item How well did the simulation depict the resistance and friction of the guidewire against the walls of the vessel?
% \item How realistic were the visual representations of the guidewire's interaction with the vessel walls?
% \item How closely did the guidewire's motion match your expectations of how a real guidewire would move?
% \item How visually realistic was the guidewire simulation?
% \end{enumerate}



% \section{Traditional Path Planning}
% \label{app_path_planning}

% To emphasize our choice of using a neural network policy as the expert, we conducted a defining experiment. We initially used the A* planner~\citep{hart1968formal} to identify the most straightforward route from a starting position to the goal, ensuring sampling was restricted to the aortic arch. This plan is depicted in Fig.~\ref{fig:path-planning}. However, the results revealed that the shortest path is not always the best. The cannulation efficiency along this route was suboptimal, and there was no standardized method to determine the exact actuation for the guidewire tip to follow this path. Expanding our research, we utilized a Multilayer Perceptron (MLP) to predict the next action from a sequence of observations. Yet, this model also faced difficulties in following the desired route, highlighting the intrinsic complexities of the task. The agent's actual path, showing the guidewire's deviation, can be seen below:

% \begin{figure}[h]
%     \centering
%     \includegraphics{assets/rebuttal/path_following.png}
%     \caption{Path Planning}
%     \label{fig:path-planning}
% \end{figure}

% \section{Shape Prediction}
% \label{app_shape_pred}


% Shape prediction, especially for guidewires, is instrumental in reducing vasculature stress and optimizing control performance. This ultimately results in a substantial reduction in complication risks~\citep{shi2016shape}. Efforts to attain precise shape prediction have led to significant investments in shape-sensing technologies. One noteworthy example is the FBG-sensors~\citep{chitalia2020towards}, tailored for shape approximation. However, the incorporation of these sensors presents several challenges. They not only entail material costs and augment the instrument size but also limit navigational abilities and necessitate major alterations to optimize guidewire features, including stiffness. To navigate these environments, alternatives have been sought, including reconstructions from bi-planar scanner images or those anchored in precise kinematics~\citep{shi2016shape}. While deep learning emerges as a promising solution, especially in terms of cost mitigation, it inherently demands extensive data.

% \begin{figure}[h]
%     \centering
%     \subfigure{\includegraphics{assets/rebuttal/shape_prediction.png}}
%     \caption{Shape Prediction}
%     \label{fig:shape}
% \end{figure}

% We posit that our simulator can be instrumental in furnishing the necessary data to train models that use images to approximate instrument shapes. To affirm this, we have juxtaposed image observations of shape $80\times80$ with the real 3D positions of the guidewire bodies $p$, facilitating the guidewire shape reconstruction from 2D images. Using this data, we trained a CNN, leveraging the NAdam optimizer~\citep{dozat2016incorporating} and a refined loss function encompassing the Huber Loss~\citep{huber1992robust} with a $\delta=1$:

% \begin{equation}
% \mathcal{L}_{\text{Huber}}(y, \hat{y}) = \begin{cases} 
%                                     \frac{1}{2}(y - \hat{y})^{2} & \text{if } \left | y - \hat{y} \right | < \delta \\
%                                     \delta \left( \left| y - \hat{y} \right| - \frac{\delta}{2} \right) & \text{, otherwise}
%                                 \end{cases}\,,
% \end{equation}

% Here, $y$ denotes the ground truth positions of the guidewire bodies, and $\hat{y}$ signifies the predicted positions. A regularization term, $\mathcal{L}_{\text{reg}}$, is introduced to ensure the guidewire's geometric structure remains intact, assuming an interbody distance of $2\unit{mm}$:

% \begin{equation}
%     \mathcal{L}_{\text{reg}} = \frac{1}{n-1} \sum_{i=1}^{n-1} \left| \lVert \hat{y}_{i+1} - \hat{y}_i \rVert_2 - 0.002 \right|
% \end{equation}

% The combined loss is then represented as:

% \begin{equation}
%     \mathcal{L}= \alpha \mathcal{L}_{\text{Huber}}(y, \hat{y}) + \beta \mathcal{L}_{\text{reg}}\,,
% \end{equation}

% Our comparative analysis between the actual guidewire shape and its prediction is visually represented in Fig.~\ref{fig:shape}. The close approximation of the guidewire shape from the 2D image underscores our simulator's potential. 

% Such findings highlight the capacity of our simulator to enhance auxiliary tasks, enabling researchers to utilize the simulator for data-driven model samples. While this provides a foundation, a deeper delve into simulation to real transfer nuances is warranted in future research. Nevertheless, considering the exorbitant costs of real-world data acquisition, our simulator stands out as a pivotal tool in the evolution of these methodologies.



% \section{Network Choice}\label{app:network-choice}

% In our experimental trials, we implemented a transformer-based architecture, drawing inspiration from the visual transformer by~\cite{dosovitskiy2020image}. This architecture was specifically tailored with an image size of \(80\), a patch size of \(10\), and a single-channel configuration, alongside a depth of \(3\) and \(4\) heads within the attention layers. Despite these specifications, the transformer model did not achieve the expected performance level in our specialized domain of endovascular navigation. It notably struggled to complete the designated tasks within the desired timeframe. This underperformance, coupled with signs of convergence, is illustrated in Fig~\ref{app-fig:vit}, highlighting the challenges encountered in applying this model to our specific context.

% \begin{figure}[h]
%     \centering
%     \includegraphics{assets/rebuttal/vit.png}
%     \caption{\textbf{ViT-Based ENN Trials:} Initial results indicate that using ViT as a feature extractor does not improve outcomes and fails to meet the target within the time limit, despite showing convergence.}
%     \label{app-fig:vit}
% \end{figure}


% \section{Sim-to-Real Imaging Gap}

% We showcase the adaptability of our endovascular simulator using domain adaptation techniques. This is crucial for translating simulated environments into more realistic, X-ray-like images. The implementation of this approach is based on the work of~\cite{kang2023translating}. Their method, employing multi-scale semantic matching, effectively ensures the preservation of essential structural information in medical images while transitioning from simulated to real-world imaging styles. This technique has demonstrated significant success in producing realistic X-ray images and has set a new benchmark in the field. For an in-depth understanding and visual representation of this adaptation process, we refer readers to the detailed findings and illustrations in the work of~\cite{kang2023translating}. The adapted images can be visualized in Fig.~\ref{app-fig:sim2real}.

% \begin{figure}[h]
% \centering
% \subfigure[]{\includegraphics[width=0.28\linewidth, height=0.28\linewidth]{assets/sim2real/0.png}}
% \hspace{1px}
% \subfigure[]{\includegraphics[width=0.28\linewidth, height=0.28\linewidth]{assets/sim2real/1.png}}
% \hspace{1px}
% \subfigure[]{\includegraphics[width=0.28\linewidth, height=0.28\linewidth]{assets/sim2real/2.png}}
% \vspace{-1ex}
% \caption{\textbf{Sim-to-Real Adaptation:} Demonstration of sim-to-real domain adaptation for creating realistic renderings, featuring \textit{a)} the input image, \textit{b)} the resultant generated image, and \textit{c)} a real X-ray image example. Figure addapted from~\cite{kang2023translating}}
% \label{app-fig:sim2real}
% \end{figure}
